# Supplementary material for: IntereStyle: Encoding an Interest Region for Robust StyleGAN Inversion
Source: arXiv:2209.10811 source file (2022-11-15)
Supplement: Supplementary file 1 [file X_supplementary.tex]

\appendix

% --- PDF will be split by an editor (e.g. macOS preview), so need to restart from page 1
\setcounter{page}{0}

% --- repeat the title (AT: haven't found a more elegant way to do this...)
\clearpage

% \vspace{0.5em}Supplementary Material \\
%< twocolumn

\section{Training Details}
\label{app:training}

\section{Dataset description}

\section{Baseline models description}
\label{app:baselines}

\section{Qualitative results}
\label{app:qualitative}
\subsection{Inversion Results}
\label{app:inversion}

\subsection{Editing via Latent Manipulations}
\label{app:interpolation}

\section{Limitations}
\label{app:limitations}

\section{Potential Negative Societal Impacts}
